# Supplementary material for: EVE: Efficient Verification of Data Erasure through Customized Perturbation in Approximate Unlearning
Source: arXiv:2602.03567 source file (2026-02-03)
Supplement: Supplementary file 1 [file appendix2.tex]

\subsection{Unlearning Effect Guarantee by Incremental Training} \label{training_details_appendix}

\begin{figure}[h]
	\centering
	\hspace{-5mm}
	\subfloat[On CIFAR10]{ 	\label{fig:cifar10accduringtraining} 
		\includegraphics[scale=0.34]{../../../../PycharmProjects/OUL/Experimental_results/On_CIFAR10/Model_acc/cifar10_acc_during_training}
	}			
	\hspace{-3mm}
	\subfloat[On CelebA]{ 	\label{fig:celebaaccduringtraining} 
		\includegraphics[scale=0.34]{../../../../PycharmProjects/OUL/Experimental_results/On_CelebA/Model_acc/CelebA_acc_during_training}
	}			
	\caption{Training Details on CIFAR10 and CelebA} %\vspace{-2mm}
	\label{details_during_training} 
\end{figure}

\begin{figure*}[h]
	\centering
	\hspace{-5mm}
	\subfloat{ 	\label{fig:mnistorgsimnoiseanalysis}  \rotatebox{90}{ \hspace{8mm}	\scriptsize{ On MNIST} }
		\includegraphics[scale=0.24]{../../../../PycharmProjects/OUL/Experimental_results/On_MNIST/Original_sim/mnist_org_sim_noise_analysis}
	}			
	\hspace{-3mm}
	\subfloat{  \label{fig:mnistforgeabilityunlsim}
		\includegraphics[scale=0.24]{../../../../PycharmProjects/OUL/Experimental_results/On_MNIST/Forgeability/mnist_forgeability_unl_sim}
	} 
	\hspace{-3mm}
	\subfloat{\label{fig:mnistmodelaccunlsim}  
		\includegraphics[scale=0.24]{../../../../PycharmProjects/OUL/Experimental_results/On_MNIST/Model_acc/mnist_model_acc_unl_sim}
	}			
	\hspace{-3mm}
	\subfloat{ 		\label{fig:mnistbackaccunlsim}
		\includegraphics[scale=0.24]{../../../../PycharmProjects/OUL/Experimental_results/On_MNIST/Back_acc/mnist_back_acc_unl_sim}
	}
	\hspace{-3mm}
	\subfloat{  		\label{fig:mnistreconsimunlsim}
		\includegraphics[scale=0.24]{../../../../PycharmProjects/OUL/Experimental_results/On_MNIST/Recon_sim/mnist_recon_sim_unl_sim}
	}\vspace{-3mm} \\
	\hspace{-5mm}
	\subfloat{ 	  	\label{fig:cifar10orgsimnoiseanalysis} \rotatebox{90}{ \hspace{8mm}	\scriptsize{ On CIFAR10} }
		\includegraphics[scale=0.24]{../../../../PycharmProjects/OUL/Experimental_results/On_CIFAR10/Original_sim/cifar10_org_sim_noise_analysis}
	}			
	\hspace{-3mm}
	\subfloat{  \label{fig:cifar10forgeabilityunlsim}
		\includegraphics[scale=0.24]{../../../../PycharmProjects/OUL/Experimental_results/On_CIFAR10/Forgeability/cifar10_forgeability_unl_sim}
	} 
	\hspace{-3mm}
	\subfloat{ 	 	\label{fig:cifar10modelaccunlsim}  
		\includegraphics[scale=0.24]{../../../../PycharmProjects/OUL/Experimental_results/On_CIFAR10/Model_acc/cifar10_model_acc_unl_sim}
	}			
	\hspace{-3mm}
	\subfloat{ 	 	\label{fig:cifar10backaccunlsim}
		\includegraphics[scale=0.24]{../../../../PycharmProjects/OUL/Experimental_results/On_CIFAR10/Back_acc/cifar10_back_acc_unl_sim}
	}
	\hspace{-3mm}
	\subfloat{    	\label{fig:cifar10reconsimunlsim}
		\includegraphics[scale=0.24]{../../../../PycharmProjects/OUL/Experimental_results/On_CIFAR10/Recon_sim/cifar10_recon_sim_unl_sim}
	} \vspace{-3mm}  \\
	\hspace{-5mm}
	\subfloat{		\label{fig:celebaorgsimnoiseanalysis} \rotatebox{90}{ \hspace{8mm}	\scriptsize{ On CelebA} }
		\includegraphics[scale=0.24]{../../../../PycharmProjects/OUL/Experimental_results/On_CelebA/Original_sim/celebA_org_sim_noise_analysis}
	}	
	\hspace{-3mm}
	\subfloat{ 	\label{fig:celebaforgeabilityunlsim}
		\includegraphics[scale=0.24]{../../../../PycharmProjects/OUL/Experimental_results/On_CelebA/Forgeability/CelebA_forgeability_unl_sim}
	} 		
	\hspace{-3mm}
	\subfloat{	\label{fig:celebamodelaccunlsim}  
		\includegraphics[scale=0.24]{../../../../PycharmProjects/OUL/Experimental_results/On_CelebA/Model_acc/CelebA_model_acc_unl_sim}
	}			
	\hspace{-3mm}
	\subfloat{ 		\label{fig:celebabackaccunlsim}
		\includegraphics[scale=0.24]{../../../../PycharmProjects/OUL/Experimental_results/On_CelebA/Back_acc/CelebA_back_acc_unl_sim}
	}
	\hspace{-3mm}
	\subfloat{  		\label{fig:celebareconsimunlsim}
		\includegraphics[scale=0.24]{../../../../PycharmProjects/OUL/Experimental_results/On_CelebA/Recon_sim/CelebA_recon_sim_unl_sim}
	}%\vspace{-2mm}
	\caption{Evaluations for the impact of unlearning samples' similarity} %\vspace{-2mm}
	\label{evaluation_of_unl_sim} 
\end{figure*}

We have shown the detailed training process on MNIST in \Cref{fig_mnistaccduringtraining} to illustrate the effectiveness of OUbL. This section shows the supplementary experimental results of training details on CIFAR10 and CelebA. Results on both datasets confirm the unlearning effectiveness via incremental training of OUbL.
 
 \vspace{2mm}
 \noindent
\textbf{Setup.}
We first recall our experimental setup. We conduct the incremental training on the clean dataset and the constructed dataset $D_{a}^p$, which is synthesized by OUbL. In the experiment, we set the unlearning size ratio $\text{\it USR}=1\%$, and the size ratios of clean data and auxiliary data, $\text{\it CSR} =1\%$ and $\text{\it ASR} =1\%$. The experimental results are presented in \Cref{details_during_training}. 

\vspace{2mm}
\noindent
\textbf{Analysis of the Unlearning Effectiveness via Incremental Training.} 
The \Cref{details_during_training} illustrates the backdoor accuracy (data removal effect) over 40 training rounds for two different datasets: CIFAR10 and CelebA. The plots compare the performance between clean data and synthesized data using the OUbL method.

For the training on clean data, the backdoor accuracy remains consistently high, close to 100\% on CIFAR10 and above 60\% on CelebA, across all 40 training rounds. This indicates that the model still retains the backdoor when trained on clean data.

For the incremental train on the synthesized data via OUbL, the backdoor accuracy drops sharply to near 0\% after the initial training rounds and remains low with slight fluctuations throughout the remaining rounds on both CIFAR10 and CelebA. This suggests that the OUbL method effectively achieves data removal via incremental training using the synthesized data.

Therefore, the incremental training of the OUbL method shows a significant reduction in backdoor accuracy for both CIFAR10 and CelebA datasets, indicating its effectiveness in unlearning. Training on clean data, on the other hand, maintains high backdoor accuracy, highlighting the contribution of the unlearned samples still existing on the model.

\subsection{Impact of Unlearning Samples Similarity} \label{additional_ablation}

%\noindent
%\textbf{Impact of Unlearning Samples Similarity}

We know that the similarity between the erased samples and the remaining samples plays an important role in machine unlearning. In this section, we also conduct experiments to evaluate how the similarity influences the performance of OUbL.

\vspace{2mm}
\noindent
\textbf{Setup.} To quantify the similarity between the erased samples and the remaining samples, we introduce a backdoor ratio $\beta$ to control the injected patch to the erased samples, formulated as $D_{u, \beta} \gets (X_u + \beta \times patch, Y_u)$. We mixed both $D_{u,\beta}$ and original unlearned data $D_u$ into the training dataset for ML service model training. During the unlearning process, we only need to remove the contribution of the marked samples $D_{u, \beta}$. By adjusting $\beta$, we can simulate the different levels of similarity between the erased samples and the samples in the remaining dataset. This approach allows us to intuitively quantify the similarity between the unlearned samples and the remaining samples. The experimental results on MNIST, CIFAR10 and CelebA are presented in \Cref{evaluation_of_unl_sim}. 

\vspace{1mm}
\noindent
\textbf{Relationship between Unlearned Data Similarity and Patch Injection Ratio.} The first column in \Cref{evaluation_of_unl_sim} illustrates the relationship between the patch injection ratio $\beta$ and similarity, where similarity is measured between the original samples $D_u$ and the patch-injected data $D_{u, \beta}$. In this experiment, we only need to unlearn $D_{u\beta}$. Across all datasets, including MNIST, CIFAR10, and CelebA, increasing the amount of noise (as indicated by a higher $\beta$) results in a decrease in similarity. This trend is consistently observed, demonstrating that higher patch injection ratios make the unlearned samples more distinct from the original samples in the remaining dataset.

\vspace{1mm}
\noindent
\textbf{Impact on Unlearning Update Similarity.}
The second column in \Cref{evaluation_of_unl_sim} demonstrates the unlearning update similarity influenced by the patch ratio $\beta$. With more patches injected into the data, the marked samples will be more dissimilar to the original samples and the remaining samples. It increases the difficulty of OUbL in approaching the unlearning update via incremental learning, as the normal clean and the auxiliary data that we can use are not similar to the unlearned samples with a high patch injecting ratio. The unlearning update similarity obviously decreases as the patch ratio increases on all three datasets.

\vspace{1mm}
\noindent
\textbf{Impact on Unlearning Effectiveness.}
The third and fourth columns demonstrate the model utility and data removal of unlearning effectiveness. The data removal effect increases as the patch ratio increases, showing as the decreased backdoor accuracy. It means the more unique samples, larger $\beta$ and lower similarity, are easier to be unlearned. However, better data removal effect slightly decreases model utility, as showing from the model accuracy of all methods in the third column in \Cref{evaluation_of_unl_sim}.

\vspace{1mm}
\noindent
\textbf{Impact on Erased Data Protection.}
Our OUbL achieves the best privacy protection for the erased samples, and the attacking difficulty for OUbL increases as the patch ratio increases. It is easy to understand because OUbL is more difficult to forge the unlearning update when patch ratio increases, which means the constructed data contains less unqiue information about the erased samples when $\beta$ is large. It makes the unlearning update less similar to the expected ones, and hence increase the reconstruction difficulty.

We omit the illustration of the unlearning efficiency results as the similarity not heavily influence the training time.

%\noindent
%\textbf{Impact on Unlearning Efficiency.}

\begin{tcolorbox}[colback=white, boxrule=0.3mm]
	\noindent \textbf{Takeaway 6.}  As the patch ratio increases, the similarity between the unlearned samples and the remaining dataset decreases, making the unlearned samples more unique. Consequently, OUbL finds it more challenging to approach the unlearning update with a higher patch ratio, which reduces the model's utility to some extent. At the same time, this increased uniqueness makes the model harder to be attacked by reconstruction attacks. 
\end{tcolorbox}
