# Supplementary material for: EVE: Efficient Verification of Data Erasure through Customized Perturbation in Approximate Unlearning
Source: arXiv:2602.03567 source file (2026-02-03)
Supplement: Supplementary file 3 [file appendix10.tex]

\subsection{Costs Associated With Storage}
\label{app:storage}

\new{The slicing introduced by \SISA is trading disk storage for unlearning speed-up. This is supported by the fact that the the cost of GPU accelerators is more than the cost of storage disks. For instance, storage costs \$0.026/Gb/Month on Google Cloud, \$0.023/Gb/Month on Amazon Web Services, and \$0.058/GB per month on Azure at the time of writing. Instead, renting the cheapest GPUs starts at \$0.25/hour on Google Cloud, \$0.526/hour on Amazon Web Services, and \$0.90/hour on Azure. 
To limit usage of GPU accelerators, it is already a common practice to regularly checkpoint models during training. Hence, we believe the overhead from slicing will not be a drawback: in most cases, it will suffice to change the order in which data is presented during training because checkpointing is already in place.}
