# Supplementary material for: EVE: Efficient Verification of Data Erasure through Customized Perturbation in Approximate Unlearning
Source: arXiv:2602.03567 source file (2026-02-03)
Supplement: Supplementary file 8 [file appendix7.tex]

\subsection{Lone Shard Baseline Time Analysis}
\label{appendix:time_baseline}

\noindent{\bf Definition:} A lone shard is a model trained on a $\frac{1}{S}$ fraction of the dataset. The remainder of data is not used for training.

\subsubsection{Sequential Setting}
\label{appendix:seq_lon_shard}

\noindent

\noindent\emph{1. Assumption:} The assumptions made in Appendix~\ref{appendix:time_sharding_sequential} are valid here, though we only have one shard of initial size $\frac{N}{S}$. The probability of it being impacted is approximately equal to $\frac{1}{S}$.

\noindent\emph{2. Size of the retraining set:} We can develop a reasoning very similar to Appendix~\ref{appendix:time_sharding_sequential}. At each step, two cases are possible. Either we affect a shard, the only shard we have. This corresponds to the event $E_{i,j}$ of Appendix~\ref{appendix:time_sharding_sequential} if the shards has already been affected $j$ times, or we affect no shard with cost $0$. We call this event $Z_i$.

\noindent\emph{3. Associated probabilities:}
The probability of $Z_i$, since we have only one shard, is $1 - \frac{1}{S}$. Notice that in Appendix~\ref{appendix:time_sharding_sequential} this event had zero probability.
The probability of $E_{i,j}$ is $\frac{1}{S}{i - 1 \choose j}\left(\frac{1}{S}\right)^{j}\left(\frac{1}{S}\right)^{i - 1 - j}$. The factor $\frac{1}{S}$ accounts for the fact that request $i$ affects a shard with probability $\frac{1}{S}$, the rest of the formula is similar to the one in Appendix~\ref{appendix:time_sharding_sequential}.

\noindent\emph{4. Expected cost:}
We can easily show that we obtain a formula for the expected cost similar to the one in Appendix~\ref{appendix:time_sharding_sequential} but with a $\frac{1}{S}$ factor:
\begin{equation}\mathbb{E}[C] = \frac{1}{S}\left(\frac{N}{S} + \frac{1}{2S}-1\right)K - \frac{K^2}{2S^2}\end{equation}
Thus the lone shard baseline provides a $S\times$ speed up w.r.t. \SISA. However, this fact should not discourage the use of \SISA since the lone shard baseline will perform poorly in terms of accuracy on complex learning tasks.

\subsubsection{Batched Setting}

Let $K$ denote the batch size. We model whether the $i^{th}$ request of the batch affects the training set (or not) by a Bernoulli random variable $\mathfrak{h}_i \sim B(\frac{1}{S})$ i.i.d. We define $\mathfrak{s}_K = \sum_i{\mathfrak{h}_i}$ the number of times the shard is affected for the batch. By construction, $\mathfrak{s}_K \sim B(K,\frac{1}{S})$.
The number of points to retrain when the batch is processed is simply the total number of points in the training set minus the number of times the shard is affected: $C = \frac{N}{S} - \mathfrak{s}_K$. Thus:
{\small\begin{equation}
\mathbb{E}[C] = \frac{N-K}{S}
\end{equation}}

Recall that the batched cost of \SISA is:
{\small\begin{equation}
\mathbb{E}[C] = N\left(1-\left(1-\dfrac{1}{S}\right)^K\right) -K
\end{equation}}

For $K \ll N$, we roughly have a cost of $N(1-\exp({\frac{-K}{\tau})})$ where $\tau = (-\ln({1-\frac{1}{S}}))^{-1}$ for \SISA.

Thus for small enough $K$, there {\em might exist} a regime where \SISA outperforms the lone shard baseline. Determining a usable value of $K$ in that regime is the challenge -- $K$ can not be less than 1. Note that $K=1$ is exactly the first step of the sequential setting: the lone shard baseline provides a $S\times$ speed up w.r.t. \SISA (refer \S~\ref{appendix:seq_lon_shard}). It turns out this regime is impractical. Therefore, for small values of $K$, the lone shard baseline outperforms \SISA with a speed-up of at least $S \times$. Once again, those findings must be considered along with their impact on accuracy, and are meaningless by themselves.
